# Supplementary material for: The SP theory of intelligence: an overview
Source: arXiv:1306.3888 ancillary file (2015-01-07)
Supplement: Supplementary file 1 [file sp_in_brief.pdf]

# The SP theory of intelligence and the SP machine, in brief

J Gerard Wolff\*

January 1, 2015

“There is nothing more practical than a good theory”,  
Kurt Lewin [6].

## 1 Overview

- *Simplification and integration.* The *SP theory of intelligence* is a unique attempt to simplify and integrate concepts across artificial intelligence, mainstream computing, mathematics, and human perception and cognition, with information compression as a unifying theme.<sup>1</sup>
- *SP computer model and SP machine.* The SP theory is realised in the SP70 computer model which may be regarded as a first version of the *SP machine*.
- *Extensive development and testing.* The SP theory was not dreamed up overnight. It is the product of about 17 years of development, with testing at every stage via successive versions of the SP computer model. Many seemingly-promising ideas have been rejected as a result of this testing.

---

\*Dr Gerry Wolff, BA (Cantab), PhD (Wales), CEng, MBCS (CITP); CognitionResearch.org, Menai Bridge, UK; jgw@cognitionresearch.org; +44 (0) 1248 712962; +44 (0) 7746 290775; *Skype*: gerry.wolff; *Web*: www.cognitionresearch.org.

<sup>1</sup>The name “SP” is short for *Simplicity* and *Power*, because compression of any given body of information, **I**, may be seen as a process of reducing “redundancy” of information in **I** and thus increasing its “simplicity”, whilst retaining as much as possible of its non-redundant descriptive and explanatory “power”.

- *Publications.* The theory is described most fully in [15] and more briefly but quite fully in [17]. Potential benefits and applications are described in [20] (how the SP theory may help to solve problems associated with big data), [18] (application of the SP theory to the understanding of natural vision and the development of computer vision), [19] (application of the SP theory in the development of the ‘brains’ of autonomous robots), [14] (application of the SP system to medical diagnosis), and [16] (the SP system as an intelligent database), and [22] (several other potential areas of application including unsupervised learning, natural language processing, software engineering, information compression, the semantic web, bioinformatics, and data fusion).
- *Potential value.* In view of the wide scope of the SP system, and evidence of its potential, it seems reasonable to estimate that it could add at least 5% to the value of IT investments, worldwide. Since these are about \$3.8 trillion annually,<sup>2</sup> the value of the SP concepts, *every year*, would be at least \$190 billion! [22, Section 8].
- *A high-parallel version of the SP machine.* It is envisaged that the SP computer model will be the basis for the creation of an open-source, high-parallel version of the SP machine, hosted on an existing high-performance computer. This would be a means for researchers everywhere to explore what can be done with the system and to create new versions of it. How things may develop is shown schematically in Figure 1.

## 2 Distinctive features and apparent advantages of the SP system

Information compression and concepts of probability are themes in other research, including research on Bayesian inference, Kolmogorov complexity, deep learning, artificial neural networks, minimum length encoding, unified theories of cognition, natural language processing and more. The main features that distinguish the SP theory from these other areas of research, and apparent advantages compared with these other approaches, are:

---

<sup>2</sup>See, for example, “Gartner: Big data will help drive IT spending to \$3.8 trillion in 2014”, *InfoWorld*, 2013-01-03, [bit.ly/Z00SBr](http://bit.ly/Z00SBr).



- *The SP theory is a theory of computing.* Most other research is founded on the idea that computing may be understood in terms of the Universal Turing Machine or equivalent models such as Lamda Calculus or Post’s Canonical System. By contrast, *the SP theory is itself a theory of computing* [15, Chapter 4].
- *Intelligence.* What is distinctive about the SP theory as a theory of computing is that it provides much of the human-like intelligence that is missing from earlier models.<sup>3</sup>
- *Information compression via the matching and unification of patterns.* In trying to cut through complexities, the SP programme focuses on a simple, ‘primitive’ idea: that information compression may be understood as a search for patterns that match each other, with the merging or ‘unification’ of patterns that are the same.
- *Multiple alignment.* More specifically, information compression via the matching and unification of patterns provides the basis for a concept of *multiple alignment*, borrowed and adapted from that concept in bioinformatics. Developing this idea as a framework for the simplification and integration of concepts across a broad canvass has been a major undertaking. *Multiple alignment is a distinctive and powerful idea in the SP programme.*
- *Transparency in the representation and processing of knowledge.* By contrast with sub-symbolic approaches to artificial intelligence, and notwithstanding objections to symbolic AI,<sup>4</sup> knowledge in the SP system is transparent and open to inspection, and likewise for the processing of knowledge.
- *SP-neural.* The SP theory includes proposals—SP-neural—for how abstract concepts in the theory may be realised in terms of neurons and neural processes. The SP-neural proposals are significantly different from artificial neural networks as commonly conceived in computer science, and arguably more plausible in terms of neuroscience.

---

<sup>3</sup>Although Alan Turing saw that computers might become intelligent [10], the Universal Turing Machine, in itself, does not tell us how! The SP theory, as it is now, goes some way towards plugging the gap, and has potential to do more. Much the same may be said about “neural Turing machines” [4] and recurrent neural networks but, with each alternative, there is room for debate about how close it gets us to the heart of “intelligence”.

<sup>4</sup>See, for example, “Hubert Dreyfus’s views on artificial intelligence”, *Wikipedia*, [bit.ly/1hGHVm8](http://bit.ly/1hGHVm8), retrieved 2014-08-19.

### 3 Outline of the SP theory and SP machine

The SP theory is conceived as an abstract brain-like system that, in an ‘input’ perspective, may receive *New* information via its senses, and compress some or all of it to create *Old* information, as illustrated schematically in Figure 2. In the theory, information compression is the mechanism both for the learning and organisation of knowledge and for pattern recognition, reasoning, problem solving, and more.

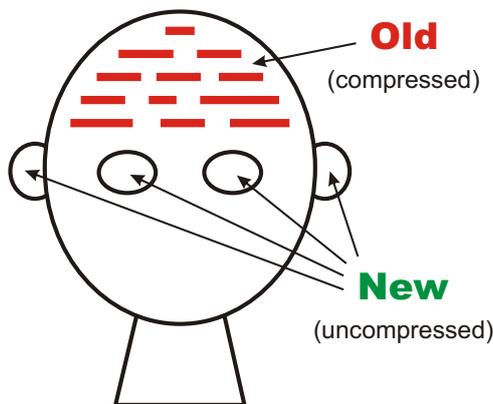

Figure 2: Schematic representation of the SP system from an ‘input’ perspective.

The subsections that follow outline the main elements of the SP theory and the SP machine.

#### 3.1 Patterns and symbols

In the SP system, knowledge is represented with arrays of atomic symbols in one or two dimensions called *patterns*. The SP70 model works with 1D patterns but it is envisaged that the system will be generalised to work with 2D patterns [17, Section 3.3].

An ‘atomic symbol’ in the SP system is simply a mark that can be matched with any other symbol to determine whether it is the same or different: no other result is permitted.

In themselves, SP patterns are not particularly expressive. But within the multiple alignment framework (Section 3.2.2), they support the representation and processing of a wide variety of kinds of knowledge (Section 4). A goal of the SP programme is to establish one system for the representation and processing of *all* kinds of knowledge (see also [20, Section III]). Evidence

to date suggests that this may be achieved with SP patterns in the multiple alignment framework.

Any collection of SP patterns is termed a *grammar*. Although that term is most closely associated with linguistics, it is used in the SP programme for a collection of SP patterns describing any kind of knowledge.

## 3.2 Information compression

In the SP theory, the emphasis on information compression derives from earlier research on grammatical inference [12] and the principle of *minimum length encoding* (MLE) [9, 11, 8]).

At an abstract level, information compression means the detection and reduction of *redundancy* in information. In more concrete terms, redundancy means *recurrent patterns*, *regularities*, *structures*, and *associations*, including *causal associations*. Thus information compression provides a means of discovering such things as words in natural language [12], objects [19, Section V-E], and associations (see, for example, [20, Section III-A.1]), in accordance with the DONSVIC principle [17, Section 5.2].<sup>5</sup>

The default assumption in the SP theory is that compression of information is always lossless, meaning that all non-redundant information is retained. In particular applications, there may be a case for discarding non-redundant information (see, for example, [20, Section X-B]) but any such discard is reversible.

In the SP system, information compression is achieved via the matching and unification of patterns. More specifically, it is achieved via the building of multiple alignments and via the unsupervised learning of grammars. These three things are described briefly in the following three subsections.

### 3.2.1 Information compression via the matching and unification of patterns

The basis for information compression in the SP system is a process of searching for patterns that match each other with a process of merging or ‘unifying’ patterns that are the same. At the heart of the SP70 model is a method for finding good full and partial matches between sequences with advantages compared with classical methods [15, Appendix A].<sup>6</sup>

---

<sup>5</sup>*DONSVIC* = “The discovery of natural structures via information compression”.

<sup>6</sup>The main advantages are [15, Section 3.10.3.1]: 1) That it can match arbitrarily long sequences without excessive demands on memory; 2) For any two sequences, it can find a set of alternative matches (each with a measure of how good it is) instead of a single ‘best’ match; 3) The ‘depth’ or thoroughness of the searching can be controlled by parameters.

### 3.2.2 Information compression via the building of multiple alignments

That process for finding good full and partial matches between patterns is the foundation for processes that build *multiple alignments* like the one shown in Figure 3.

This example shows the best multiple alignment created by the SP computer model when a set of New patterns (in column 0)<sup>7</sup> is processed in conjunction with a set of pre-existing Old patterns like those shown in columns 1 to 6. Here, the multiple alignment is ‘best’ because it is the one that achieves the most economical description of the New patterns in terms of the Old patterns. The way in which that description or ‘encoding’ is derived from a multiple alignment is explained in [15, Section 3.5] and [17, Section 4.1]. Like all other kinds of knowledge, encodings derived from multiple alignments are recorded using SP patterns (Section 3.1).

This multiple alignment may be interpreted as the result of a process of recognition (Section 4.3). The New patterns represent the features of some unknown plant and the Old patterns in columns 1 to 6 represent candidate categories, at several levels of abstraction: species ‘Meadow Buttercup’ (column 1), genus *Ranunculus* (column 6), family *Ranunculaceae* (column 5), and so on.

### 3.2.3 Information compression via the unsupervised learning of grammars

As outlined in [15, Section 3.9.2] and [17, Section 5.1], and described more fully in [15, Chapter 9], the SP system may, without assistance from a “teacher” or anything equivalent, derive one or more plausible grammars from a body of New patterns, with minimum length encoding as a guiding principle. In that process, multiple alignment has a central role as a source of SP patterns for possible inclusion in any grammar [19, Section V-B1].

### 3.2.4 Heuristic search

Like most problems in artificial intelligence, each of the afore-mentioned problems—finding good full and partial matches between patterns, finding or constructing good multiple alignments, and inferring one or more good

---

<sup>7</sup>Specifically, the New patterns in this example are ‘has\_chlorophyll’ (a pattern with one symbol), ‘<stem> hairy </stem>’, ‘<petals> yellow </petals>’, ‘<stamens> numerous </stamens>’, and ‘<habitat> meadows </habitat>’. The patterns in a set like that may be presented to the system and processed in any order.

```

0           1           2           3           4           5           6
<species>
acris
<genus> ----- <genus>
Ranunculus ----- Ranunculus
                                     <family> ----- <family>
                                     Ranunculaceae ----- Ranunculaceae
                                     <order> ----- <order>
                                     Ranunculales ----- Ranunculales
                                     <class> ----- <class>
                                     Angiospermae ----- Angiospermae
                                     <phylum> ----- <phylum>
                                     Plants ----- Plants
                                     <feeding>
has_chlorophyll ----- has_chlorophyll
                                     photosynthesises
                                     <feeding>
                                     <structure> ----- <structure>
                                     <shoot>
<stem> ----- <stem> ----- <stem>
hairy ----- hairy
</stem> ----- </stem> ----- </stem>
                                     <leaves> ----- <leaves>
                                     compound
                                     palmately_cut
                                     </leaves> ----- </leaves>
                                     <flowers> ----- <flowers>
                                     <arrangement>
                                     regular
                                     all_parts_free
                                     </arrangement>
                                     <sepals>
<sepals> ----- <sepals>
not_reflexed
</sepals> ----- </sepals>
<petals> ----- <petals> ----- <petals>
                                     <number> ----- <number>
                                     five
                                     </number> ----- </number>
                                     <colour>
yellow ----- yellow
                                     </colour>
</petals> ----- </petals> ----- </petals>
                                     <hermaphrodite>
<stamens> ----- <stamens>
numerous ----- numerous
</stamens> ----- </stamens>
                                     <pistil>
                                     ovary
                                     style
                                     stigma
                                     </pistil>
                                     </hermaphrodite>
                                     </flowers> ----- </flowers>
                                     <shoot>
                                     <root>
                                     </root>
                                     </structure> ----- </structure>
<habitat> ----- <habitat> ----- <habitat>
meadows ----- meadows
</habitat> ----- </habitat>
<common_name> ----- <common_name>
Meadow
Buttercup
</common_name> ----- </common_name>
                                     <food_value> ----- <food_value>
                                     poisonous
                                     </food_value> ----- </food_value>
                                     </phylum> ----- </phylum>
                                     </class> ----- </class>
                                     </order> ----- </order>
                                     </family> ----- </family>
</genus> ----- </genus>
</species>
0           1           2           3           4           5           6

```

Figure 3: The best multiple alignment created by the SP model, with a set of New patterns (in column 0) that describe some features of an unknown plant, and a set of Old patterns, including those shown in columns 1 to 6, that describe different categories of plant, with their parts and sub-parts, and other attributes.

grammars from a body of data—is normally too complex to be solved by exhaustive search.

With intractable problems like these, it is often assumed that the goal is to find theoretically ideal solutions. But with these and most other AI problems, “The best is the enemy of the good”. By scaling back one’s ambitions and searching for “reasonably good” solutions, it is often possible to find solutions that are useful without undue computational demands.

As with other AI applications, and as with the building of multiple alignments in bioinformatics, the SP70 model uses heuristic techniques in all three cases mentioned above. This means searching for solutions in stages, with a pruning of the search tree at every stage, guided by measures of success [15, Appendix A; Sections 3.9 and 3.10; Chapter 9]. With these kinds of techniques, acceptably good approximate solutions can normally be found without excessive computational demands and with “big O” values that are within acceptable limits.

### 3.3 Multiple alignment and the representation and processing of diverse kinds of knowledge

The expressive power of SP patterns within the multiple alignment framework derives in large part from the way that symbols in one pattern may serve as links to one or more other patterns or parts thereof. One of several examples in Figure 3 is how the pair of symbols ‘<family> ... </family>’ in column 6 serves to identify the pattern ‘<family> ... Ranunculales ... <hermaphrodite> ... poisonous ... </family>’ in column 5.

In the figure, these kinds of linkages between patterns mean that the unknown plant (with characteristics shown in column 0) may be recognised at several different levels within a hierarchy of classes: genus, family, order, class, and so on. Although it is not shown in this example, the system also supports cross classification.

In the figure, the parts and sub-parts of the plant are shown in such structures as ‘<shoot>’ (column 3), ‘<flowers>’ (column 5), ‘<petals>’ (column 6), and so on.

As in conventional systems for object-oriented design, the system provides for inheritance of attributes (Section 4.6). But unlike such systems, there is smooth integration of class hierarchies and part-whole hierarchies, without awkward inconsistencies [16, Section 4.2.1].

More generally, SP patterns within the multiple alignment framework provide for the representation and processing of a wide variety of kinds of knowledge including: the syntax and semantics of natural language; class

hierarchies and part-whole hierarchies (as just described); networks and trees; entity-relationship structures; relational knowledge; rules and several kinds of reasoning; patterns and pattern recognition; images; structures in three dimensions; and procedural knowledge. There is a summary in [20, Section III-B], and more detail in Section 4.

### 3.4 Information compression, prediction, and probabilities

Owing to the close connection between information compression and concepts of prediction and probability [7], the SP system is fundamentally probabilistic. Each SP pattern has an associated frequency of occurrence and probabilities may be calculated for each multiple alignment and for any inference that may be drawn from any given multiple alignment.

### 3.5 SP-neural

Part of the SP theory is the idea, described most fully in [15, Chapter 11], that the abstract concepts of *symbol* and *pattern* in the SP theory may be realised more concretely in the brain with collections of neurons in the cerebral cortex.

The neural equivalent of an SP pattern is called a *pattern assembly*. The word “assembly” has been adopted in this term because the concept is quite similar to Donald Hebb’s [5] concept of a *cell assembly*. The main difference is that the concept of pattern assembly is unambiguously explicit in proposing that the sharing of structure between two or more pattern assemblies is achieved by means of ‘references’ from one structure to another, as described and discussed in [15, Section 11.4.1]).

It is pertinent to mention that unsupervised learning in the SP theory ([15, Chapter 9], [17, Section 5]) is quite different from “Hebbian learning” as described by Hebb [5] and widely adopted in the kinds of artificial neural networks that are popular in computer science.<sup>8</sup> By contrast with Hebbian learning, the SP system, like a person, may learn from a single exposure to some situation or event. And, by contrast with Hebbian learning, it takes time to learn a language in the SP system because of the complexity of the search space, not because of any kind of gradual strengthening or “weighting” of links between neurons [15, Section 11.4.4].

Figure 4 shows schematically how pattern assemblies may be represented and inter-connected with neurons. Here, each pattern assembly, such as ‘<

---

<sup>8</sup>See, for example, “Hebbian theory”, *Wikipedia*, [bit.ly/1sW6ATt](http://bit.ly/1sW6ATt), retrieved 2014-12-19.

NP < D > < N > >', is represented by the sequence of atomic symbols of the corresponding SP pattern. Each atomic symbol, such as '<' or 'NP', would be represented in the pattern assembly by one neuron or a small group of inter-connected neurons.<sup>9</sup> Apart from the inter-connections amongst pattern assemblies, the cortex in SP-neural is somewhat like a sheet of paper on which knowledge may be written in the form of neurons.

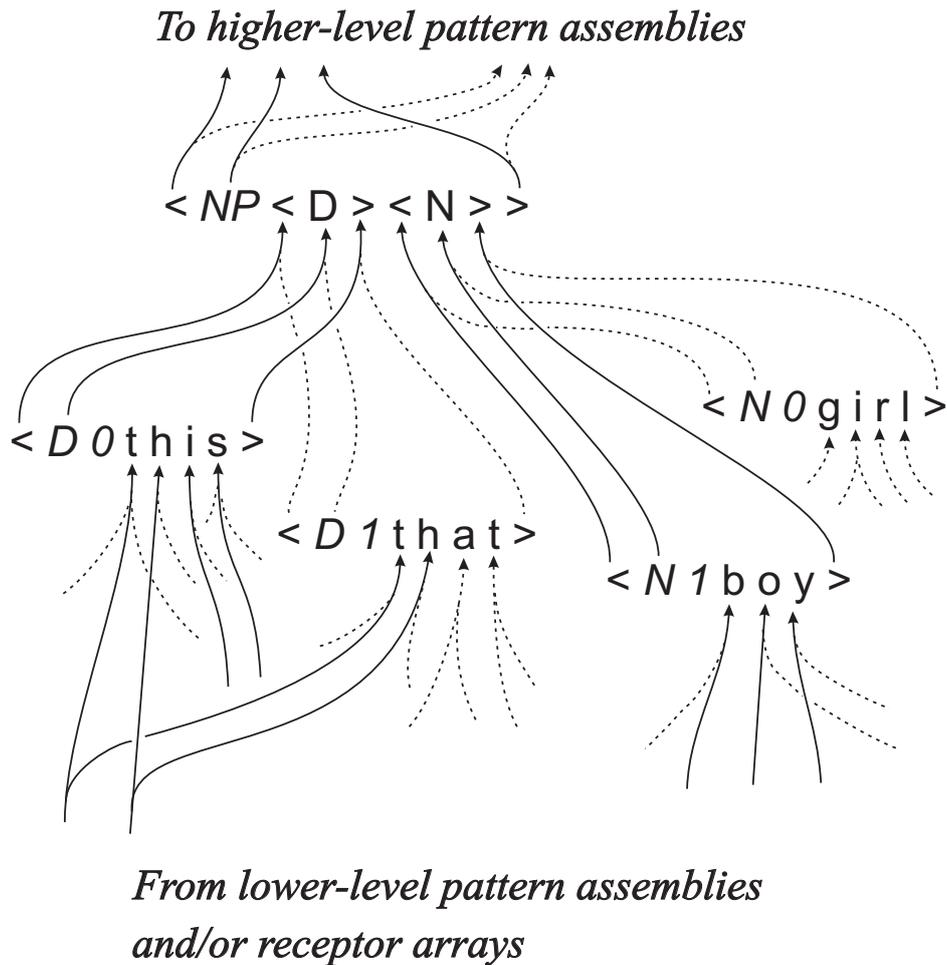

Figure 4: Schematic representation of inter-connections amongst pattern assemblies as described in the text. Not shown in the figure are lateral connections within each pattern assembly, and inhibitory connections.

It is envisaged that any pattern assembly may be 'recognised' if it receives more excitatory inputs than rival pattern assemblies, perhaps via a winner-

<sup>9</sup>Not shown in the figure are lateral connections within each pattern assembly and inhibitory connections elsewhere, as outlined in [15, Sections 11.3.3 and 11.3.4].

takes-all mechanism [15, Section 11.3.4]. And, once recognised, any pattern assembly may itself be a source of excitatory signals leading to the recognition of higher-level pattern assemblies.

## 4 Simplicity and versatility

The quest for simplification and integration in the SP theory accords with Occam’s Razor, one of the most widely-accepted principles in science. In terms of that principle—seeking to combine conceptual *simplicity* with descriptive and explanatory *power*—the SP theory scores well: a relatively simple framework provides an account of a wide range of concepts and phenomena, as outlined in the following subsections.

### 4.1 Unsupervised learning

The SP theory originates in part from an earlier programme of research on grammatical inference and the unsupervised learning of natural language, with minimum length encoding as a central principle [12], [19, Section V-A3]. However, meeting the goals of the SP programme has meant a radical reorganisation of computer models, with the development of multiple alignment as a framework for the simplification and integration of diverse structures and functions [19, Section V-A4]. The new model demonstrates capabilities in grammatical inference ([15, Chapter 9], Section 3.2.3) and appears to have considerable potential for further development, with linguistic, visual, and other kinds of knowledge.

### 4.2 Natural language processing

In addition to the learning of linguistic knowledge (Section 4.1), the SP system has strengths in the parsing of natural language, the production of natural language, and the integration of syntactic and semantic knowledge, as outlined in this section. These aspects of the system are described more fully in [17, Section 8] and in [15, Chapter 5].

#### 4.2.1 Parsing of natural language

Figure 5 shows how, via multiple alignment, a sentence (in row 0) may be parsed in terms of grammatical structures including words (rows 1 to 8).<sup>10</sup>

---

<sup>10</sup>Compared with the multiple alignment shown in Figure 3, this multiple alignment is rotated through 90°, replacing columns with rows. The choice between these two styles,

It also shows, in row 8, how the system may mark the syntactic dependency between the plural subject of the sentence (‘Np’) and the plural main verb (‘Vp’) (see also [15, Sections 5.4 and 5.5], [17, Section 8.1]).

|   |     |     |   |    |  |   |    |   |    |   |   |   |    |     |    |  |   |   |    |   |   |   |   |   |    |   |
|---|-----|-----|---|----|--|---|----|---|----|---|---|---|----|-----|----|--|---|---|----|---|---|---|---|---|----|---|
| 0 |     | t   | h | e  |  | a | p  | p | l  | e | s |   | a  | r   | e  |  | s | w | e  | e | t | 0 |   |   |    |   |
| 1 |     |     |   |    |  |   |    |   |    |   |   |   |    |     |    |  |   |   |    |   |   | 1 |   |   |    |   |
| 2 |     |     |   |    |  | N | Nr | 6 | a  | p | p | l | e  | #N  |    |  |   |   |    |   |   |   | 2 |   |    |   |
| 3 |     |     |   |    |  |   |    |   |    |   |   |   |    |     |    |  |   |   |    |   |   | 3 |   |   |    |   |
| 4 |     |     |   |    |  | N | Np | N | Nr |   |   |   | #N | s   | #N |  |   |   |    |   |   | 4 |   |   |    |   |
| 5 |     |     |   |    |  |   |    |   |    |   |   |   |    |     |    |  |   |   |    |   |   | 5 |   |   |    |   |
| 6 | S   | Num | ; | NP |  |   |    |   |    |   |   |   | #N | #NP |    |  |   |   |    |   |   | 6 |   |   |    |   |
| 7 |     |     |   |    |  |   |    |   |    |   |   |   |    |     |    |  |   |   |    |   |   | 7 |   |   |    |   |
| 8 | Num | PL  | ; |    |  |   |    |   |    |   |   |   |    |     |    |  |   | A | 21 | s | w | e | e | t | #A | 8 |

Figure 5: The best multiple alignment created by the SP model with a store of Old patterns like those in rows 1 to 8 (representing grammatical structures, including words) and a New pattern (representing a sentence to be parsed) shown in row 0.

To create a multiple alignment like the one in the figure, the system needs a grammar of Old patterns, like those shown, one per row, in rows 1 to 8 of the figure. In this example, the patterns represent linguistic structures including words.

Although SP patterns are remarkably simple, it appears that, within the multiple alignment framework, they have at least the expressive power of a context-sensitive grammar [15, Sections 5.4 and 5.5]. As previously noted (Section 3.1), there is reason to believe that all kinds of knowledge may be represented, within the multiple alignment framework, by SP patterns.

#### 4.2.2 Production of natural language

A neat feature of the SP system is that one set of mechanisms and processes may achieve both the analysis or parsing of natural language (Section 4.2.1) and the generation or production of sentences. This is explained in [15, Section 3.8] and [17, Section 4.5].

#### 4.2.3 The integration of syntax and semantics

The use of one simple format for all kinds of knowledge is likely to facilitate the seamless integration of syntax and semantics. Preliminary examples of

---

which are equivalent, depends largely on what fits best on the page.

how this may be done are shown in [15, Section 5.7], both for the derivation of meanings from surface forms [15, Figure 5.18] and for the production of surface forms from meanings [15, Figure 5.19].

#### **4.2.4 Parallel streams of information**

Up to now, most work on natural language within the SP programme has made the simplifying assumption that language may be represented with a sequence of symbols, as in ordinary text. But with some aspects of natural language such as formants in speech, and the relationship between syntax and semantics, there seem to be parallel streams of information. The way in which such parallelism may be represented and processed with 2D patterns in the SP system is described in [19, Section 4.4.4 and Appendix C].

### **4.3 Pattern recognition**

As described quite fully in [15, Chapter 6] and more briefly in [17, Section 9], the SP system has strengths in several aspects of pattern recognition:

- It can recognise patterns at multiple levels of abstraction, with the integration of class-inclusion relations and part-whole relations, as shown in the example in Figure 3.
- It can model “family resemblance” or polythetic categories, meaning that recognition does not depend on the presence absence of any particular feature or combination of features.
- Recognition is robust in the face of errors of omission, commission or substitution in the New pattern or patterns.
- For any given identification, or any related inference, the SP system may calculate associated probabilities.
- As a by-product of how recognition is achieved via the building of multiple alignments, the system provides a model for the way in which context may influence recognition.

### **4.4 Information storage and retrieval, with intelligence**

The SP theory provides a versatile model for database systems, with the ability to accommodate object-oriented structures, as well as relational ‘tuples’, and network and tree models of data [16]. It lends itself most directly

to information retrieval in the manner of query-by-example but it appears to have potential to support the use of natural language or query languages such as SQL.

Unlike some ordinary database systems:

- The storage and retrieval of information is integrated with other aspects of intelligence such as pattern recognition, reasoning, planning, problem solving, and learning—as outlined elsewhere in this document.
- The SP system provides a simple but effective means of combining class hierarchies with part-whole hierarchies, with inheritance of attributes (Section 3.3).
- It provides for cross-classification with multiple inheritance.
- There is flexibility and versatility in the representation of knowledge arising from the fact that the system does not distinguish ‘parts’ and ‘attributes’ [16, Section 4.2.1].
- Likewise, the absence of a distinction between ‘class’ and ‘object’ facilitates the representation of knowledge and eliminates the need for a ‘metaclass’ [16, Section 4.2.2].
- SP patterns provide a simpler and more direct means of representing entity-relationship models than do relational tuples [16, Section 4.2.3].

## 4.5 Vision

With generalisation of the SP system to accommodate 2D patterns, it has potential to model several aspects of natural vision and to facilitate the development of human-like abilities in artificial vision [18]. In these connections, the main strengths and potential of the SP system are:

- Low level perceptual features such as edges or corners may be identified via the multiple alignment framework by the extraction of redundancy in uniform areas in the manner of the run-length encoding technique for information compression.
- The system may be applied in the recognition of objects and in scene analysis, with the same strengths as in pattern recognition (Section 4.3).

- There is potential for the learning of visual entities and classes of entity and the piecing together of coherent concepts from fragments [18, Section 5].
- There is potential, via multiple alignment, for the creation of 3D models of objects and of surroundings [18, Section 6].
- The SP theory provides an account of how we may see things that are not objectively present in an image, how we may recognise something despite variations in the size of its retinal image, and how raster graphics and vector graphics may be unified.
- And the SP theory has things to say about the phenomena of lightness constancy and colour constancy, ambiguities in visual perception, and the integration of vision with other senses and other aspects of intelligence.

## 4.6 Reasoning

As described in quite fully in [15, Chapters 7 and 10, Section 6.4] and more selectively in [17, Section 10], the SP system lends itself to several kinds of reasoning:

- One-step ‘deductive’ reasoning.
- Abductive reasoning.
- Reasoning with probabilistic decision networks and decision trees.
- Reasoning with ‘rules’.
- Nonmonotonic reasoning and reasoning with default values.
- Reasoning in Bayesian networks, including “explaining away”.
- Causal diagnosis.
- Reasoning which is not supported by evidence.
- Inheritance of attributes in an object-oriented class hierarchy or heterarchy.

There is also potential for spatial reasoning [19, Section IV-F1] and what-if reasoning [19, Section IV-F2].

These several kinds of reasoning may work together seamlessly without awkward incompatibilities, and likewise for how they may integrate seamlessly with such AI functions as unsupervised learning, pattern recognition, and so on [22, Sections 2, 4, and 7].

For any given inference reached via any of these kinds of reasoning, the SP system may calculate associated probabilities (Section 3.4).

Although the system is fundamentally probabilistic, it may imitate the effect of logic and other ‘exact’ forms of reasoning [15, Section 10.4.5].

## 4.7 Planning and problem solving

With data about flights between different cities, represented using SP patterns, the SP computer model may find a route between any two cities (if such a route exists) and, if there are alternative routes, it may find them as well [15, Section 8.2].

Provided they are translated into textual form, the SP computer model can solve geometric analogy problems of the kind found in puzzle books and some IQ tests [15, Section 8.3], [17, Section 12].

## 4.8 Sequential and parallel procedures

Although it may not seem obvious at first sight, the multiple alignment framework can model several devices used in ordinary procedural programming, including: *procedure*, *function*, or *subroutine*; *variable*, *value* and *type*; *function with parameters*; *conditional statement*; and the means of repeating operations such as *repeat ... until* or *do ... while* [22, Section 6.6.1]. In accordance with good practice in software engineering, the SP system facilitates the integration of ‘programs’ with ‘data’. And as previously noted (Section 3.3), the SP system supports object-oriented concepts such as class hierarchies with inheritance of attributes.

In [22, Section 6.6.3], it is suggested that, since SP patterns at the ‘top’ level are independent of each other, they may serve to model processes that may run in parallel. Now it appears that a better option is to model parallel processes as parallel streams of information, represented in 2D SP patterns as described in [19, Appendix C]. The advantage of this latter scheme is that it provides the means of showing when two or more events occur at the same time and, more generally, the relative timings of events.

Within the SP system, these structures and mechanisms may serve in the representation and processing of sequential and parallel procedures from

the real world such as those required for cooking a meal, organising a party, going shopping, and so on.

Potential benefits in software engineering include the elimination of compiling or interpretation, automatic programming, benefits in verification and validation, and helping to overcome the problem of technical debt [22, Section 6.6].

## 4.9 Mathematics

Aspects of mathematics may be understood in terms of some basic techniques for information compression: *chunking-with-codes*, *schema-plus-correction*, and *run-length coding* [21], and some features of mathematics may be modelled in the SP system [15, Chapter 10].

On the strength of this evidence and some other considerations, there is reason to believe that all of mathematics may be understood in terms of information compression. There appear to be considerable implications for mathematics, and also for science—because of the importance of mathematics as a language of science.

## 4.10 Human perception and cognition, and neuroscience

Part of the inspiration for the SP theory has been earlier research on the role of information compression in the workings of brains and nervous systems [1], [2], [3], and a programme of research on the learning of a first language or languages [12]. Thus there is reason to believe that the SP theory may help to illuminate human perception and cognition.

Since the converse is true—that insights into the nature of human perception and cognition may help to inform the development of the SP theory—the two things are often considered together, as can be seen in [15], [18] and other writings about the SP system.

As outlined in Section 3.5, the SP theory includes the proposal—called *SP-neural*—that abstract concepts in the theory may be realised in terms of neurons and their interconnections [15, Chapter 11].

## 4.11 Other potential benefits and applications

The versatility of the SP system may be seen not only in the areas outlined above but in potential benefits and applications summarised in the following subsections.

### 4.11.1 Simplification and integration

In keeping with the overall goals of the SP programme—simplification and integration of concepts across artificial intelligence, mainstream computing, mathematics, and human perception and cognition—the SP machine has potential to simplify software and to promote the seamless integration of diverse structures and functions.

In the same way that a database management system or an expert-system shell provides a re-usable framework for a variety of applications, the SP system may promote an overall simplification of computing systems by reducing or eliminating the need to recreate ‘intelligence’ in diverse applications [22, Section 5].

As previously mentioned, the provision of one simple format for knowledge and one framework for the processing of knowledge promotes seamless integration of diverse structures and functions [22, Sections 2 and 7].

Like any theory that simplifies and integrates a good range of observations and concepts, the SP theory promises deeper insights and better solutions to problems than may otherwise be achieved [22, Section 6], [19, Section IV-A3].

### 4.11.2 Big data

The SP system may help to solve several problems associated with big data [20]. In brief, these problems and their potential solutions are:

- *Overcoming the problem of variety in big data.* Harmonising diverse kinds of knowledge, diverse formats for knowledge, and their diverse modes of processing, via a universal framework for the representation and processing of knowledge (UFK).
- *Learning and discovery.* The unsupervised learning or discovery of ‘natural’ structures in data.
- *Interpretation of data.* The system has strengths in areas such as pattern recognition, information retrieval, parsing and production of natural language, translation from one representation to another, several kinds of reasoning, planning and problem solving.
- *Velocity: analysis of streaming data.* The SP system lends itself to an incremental style, assimilating information as it is received, much as people do.
- *Volume: making big data smaller.* Reducing the size of big data via lossless compression can yield several benefits.

- *Transmission of data.* There is potential for substantial economies in the transmission of data by judicious separation of ‘encoding’ and ‘grammar’.
- *Energy, speed, and bulk.* There is potential for big cuts in the use of energy in computing, for greater speed of processing with a given computational resource, and for corresponding reductions in the size and weight of computers.
- *Veracity: managing errors and uncertainties in data.* The SP system can identify possible errors or uncertainties in data, suggest possible corrections or interpolations, and calculate associated probabilities.
- *Visualisation.* Knowledge structures created by the system, and inferential processes in the system, are all transparent and open to inspection. They lend themselves to display with static and moving images.

#### 4.11.3 Autonomous robots

The SP system may help in the development of the ‘brains’ of autonomous robots, meaning robots that do not depend on intelligence or power supplies, are mobile, and are designed to exhibit as much human-like intelligence as possible [19]. In brief, the problems and potential solutions are:

- *Computational efficiency, the use of energy, and the size and weight of computers.* If a robot is to be autonomous in the sense outlined above, it needs a ‘brain’ that is efficient enough to do all the necessary processing without external assistance, does not require an industrial-scale power station to meet its energy demands, and is small enough and light enough to be carried around easily—things that are difficult or impossible to achieve with current technologies.

The SP system may help: by reducing the size of data to be processed; by exploiting statistical information that the system gathers as an integral part of how it works; and via an updated version of Donald Hebb’s [5] concept of a “cell assembly”.

- *Towards human-like versatility in intelligence.* If a robot is to operate successfully in an environment where people cannot help, or where such opportunities are limited, it needs as much as possible of the versatility in intelligence that people may otherwise provide.

The SP system demonstrates versatility via its strengths in areas such as unsupervised learning, natural language processing, pattern recognition, information retrieval, several kinds of reasoning, planning, problem solving, and more.

But the SP system is not simply a kludge of different AI functions. Owing to its focus on simplification and integration of concepts in computing and cognition (Section ??), it promises to reduce or eliminate unnecessary complexity and to avoid awkward incompatibilities between poorly-integrated subsystems as indicated in Section 4.11.1.

- *Towards human-like adaptability in intelligence.* Amongst the AI capabilities of the SP system mentioned above, unsupervised learning has particular significance because of its potential as a key to human-like adaptability in intelligence and as a foundation for other kinds of learning. The current SP computer model may be augmented to allow for the learning of structures and associations in parallel streams of information, as appears to be required for unsupervised learning in autonomous robots [19, Section V-G and Appendix C].

#### 4.11.4 Medical diagnosis

The way in which the SP system may be applied in medical diagnosis is described in [14]. The expected benefits of the SP system in that area of application include:

- A format for representing diseases that is simple and intuitive.
- An ability to cope with errors and uncertainties in diagnostic information.
- The simplicity of storing statistical information as frequencies of occurrence of diseases.
- The system provides a method for evaluating alternative diagnostic hypotheses that yields true probabilities.
- It is a framework that should facilitate the unsupervised learning of medical knowledge and the integration of medical diagnosis with other AI applications.

The main emphasis in [14] is on medical diagnosis as pattern recognition. But the SP system may also be applied to causal diagnosis [15, Section 7.9], [17, Section 10.5] so that it may be possible, for example, to reason that

“The patient’s fatigue may be caused by anemia which may be caused by a shortage of iron in the diet”.

#### 4.11.5 Information compression

Since information compression is central in the workings of the SP system (Section 3.2), there is reason to believe that an industrial-strength version of the system will be useful in that area of application.

## References

- [1] F. Attneave. Some informational aspects of visual perception. *Psychological Review*, 61:183–193, 1954.
- [2] H. B. Barlow. Sensory mechanisms, the reduction of redundancy, and intelligence. In HMSO, editor, *The Mechanisation of Thought Processes*, pages 535–559. Her Majesty’s Stationery Office, London, 1959.
- [3] H. B. Barlow. Trigger features, adaptation and economy of impulses. In K. N. Leibovic, editor, *Information Processes in the Nervous System*, pages 209–230. Springer, New York, 1969.
- [4] A. Graves, G. Wayne, and I. Danihelka. Neural Turing machines. Technical report, Google DeepMind, London, UK, 2014. See [arxiv.org/pdf/1410.5401.pdf](https://arxiv.org/pdf/1410.5401.pdf) (PDF).
- [5] D. O. Hebb. *The Organization of Behaviour*. John Wiley & Sons, New York, 1949.
- [6] K. Lewin. *Field theory in social science: Selected theoretical papers by Kurt Lewin*. Tavistock, London, 1952.
- [7] M. Li and P. Vitányi. *An Introduction to Kolmogorov Complexity and Its Applications*. Springer, New York, 2009.
- [8] J. Rissanen. Paper: Modelling by the shortest data description. *Automatica IFAC*, 14:465–471, 1978.
- [9] R. J. Solomonoff. A formal theory of inductive inference. Parts I and II. *Information and Control*, 7:1–22 and 224–254, 1964.
- [10] A. M. Turing. Computing machinery and intelligence. *Mind*, 59:433–460, 1950.

- [11] C. S. Wallace and D. M. Boulton. An information measure for classification. *Computer Journal*, 11(2):185–195, 1968.
- [12] J. G. Wolff. Learning syntax and meanings through optimization and distributional analysis. In Y. Levy, I. M. Schlesinger, and M. D. S. Braine, editors, *Categories and Processes in Language Acquisition*, pages 179–215. Lawrence Erlbaum, Hillsdale, NJ, 1988. See [bit.ly/ZIGjyc](http://bit.ly/ZIGjyc).
- [13] J. G. Wolff. Computing, cognition and information compression. *AI Communications*, 6(2):107–127, 1993. See [bit.ly/XL359b](http://bit.ly/XL359b).
- [14] J. G. Wolff. Medical diagnosis as pattern recognition in a framework of information compression by multiple alignment, unification and search. *Decision Support Systems*, 42:608–625, 2006. See [bit.ly/XE7pRG](http://bit.ly/XE7pRG).
- [15] J. G. Wolff. *Unifying Computing and Cognition: the SP Theory and Its Applications*. CognitionResearch.org, Menai Bridge, 2006. ISBNs: 0-9550726-0-3 (ebook edition), 0-9550726-1-1 (print edition). Distributors, including Amazon.com, are detailed on [bit.ly/WmB1rs](http://bit.ly/WmB1rs).
- [16] J. G. Wolff. Towards an intelligent database system founded on the SP theory of computing and cognition. *Data & Knowledge Engineering*, 60:596–624, 2007. See [bit.ly/Yg2onp](http://bit.ly/Yg2onp).
- [17] J. G. Wolff. The SP theory of intelligence: an overview. *Information*, 4(3):283–341, 2013. See [bit.ly/1hz0lFE](http://bit.ly/1hz0lFE).
- [18] J. G. Wolff. Application of the SP theory of intelligence to the understanding of natural vision and the development of computer vision. *SpringerPlus*, 3(1):552, 2014. See [bit.ly/1scmpV9](http://bit.ly/1scmpV9).
- [19] J. G. Wolff. Autonomous robots and the SP theory of intelligence. 2014. Accepted for publication in *IEEE Access*. See [bit.ly/1wZBrFz](http://bit.ly/1wZBrFz).
- [20] J. G. Wolff. Big data and the SP theory of intelligence. *IEEE Access*, 2:301–315, 2014. See [bit.ly/1jGWXDH](http://bit.ly/1jGWXDH).
- [21] J. G. Wolff. Information compression, intelligence, computing, and mathematics. Technical report, CognitionResearch.org, 2014. See [bit.ly/1jEoECH](http://bit.ly/1jEoECH).
- [22] J. G. Wolff. The SP theory of intelligence: benefits and applications. *Information*, 5(1):1–27, 2014. See [bit.ly/1lcquWF](http://bit.ly/1lcquWF).
